# Supplementary material for: A time-dependent symplectic network for non-convex path planning problems with linear and nonlinear dynamics
Source: arXiv:2408.03785 source file (2024-08-07)
Supplement: Supplementary file 1 [file appendix.tex]

\section{Sanity check}\label{sec:appendix}
\textcolor{black}{
As a sanity check, we test our method on the one-dimensional harmonic oscillator. The Hamiltonian is $H(x, p) = \frac{x^2+p^2}{2}$ for any $x,p\in\R$, and the Hamiltonian ODE system is
\begin{equation}\label{eq:HODE}
\begin{dcases}
\dot{x}(s) = \nabla_{p} H(x(s), p(s)) = p(s), & s\in[0,\frac{\pi}{4}],\\
\dot{p}(s) = -\nabla_{x} H(x(s), p(s)) = -x(s), & s\in[0,\frac{\pi}{4}],\\
x(0) = 1, \\
x(\frac{\pi}{4}) = \frac{\sqrt{2}}{2}.
\end{dcases}
\end{equation}
This problem has a ground truth solution given by
\begin{equation}\label{eqt:harmonic_ocillator_true_sol}
    \begin{dcases}
    x_{true}(s) = \cos(s), \\
    p_{true}(s) = -\sin(s).
    \end{dcases}
\end{equation}
It can be verified that under the following change of coordinates
\begin{equation}\label{eq:transformation}
    \phi(x,p) = (y(x,p), q(x,p)) = \left(\arctan\left(\frac{p}{x}\right), \frac{x^2+p^2}{2}\right),
\end{equation}
the new Hamiltonian becomes $\Tilde{H}(y,q) = q$, which is state-independent. This coordinate transformation is symplectic, see \cite[Section~8.3 on p.~200]{meyer1992}. Therefore, this problem satisfies our assumption in this paper that the original Hamiltonian ODE~\eqref{eq:HODE} can be converted to a simpler one in the form of~\eqref{eqt:HamiltonianODE_yq}.}

\textcolor{black}{
We apply the SympOCNet method to solve~\eqref{eq:HODE}. Since there is no obstacle in this problem, only the residual loss and boundary loss are considered. In other words, the loss function is $\mathcal{L}$ in~\eqref{eqt:def_loss_L}.
We denote the output of the SympOCNet method by $(x_{NN}(s), p_{NN}(s))$.
The trajectory in the latent space is denoted by $(y_{NN}(s), q_{NN}(s))$, and the trained SympNet is denoted by $\varphi_\theta$. By definition, we have 
\begin{equation*}
 (x_{NN}(s), p_{NN}(s)) = \varphi_\theta(y_{NN}(s), q_{NN}(s)).   
\end{equation*}
In Fig.~\ref{fig:oscillator}, we show the comparison between the output of the SympOCNet method and the ground truth.
In the left figure, we plot the curves of $(x_{NN}(s),p_{NN}(s))$ and $(x_{true}(s),p_{true}(s))$ parameterized by the time variable $s$. It can be seen that the error of $(x_{NN}(s),p_{NN}(s))$ computed using the SympOCNet method is very small.
In the right figure, we compare the solutions in the latent space.
Note that we do not have the uniqueness of the symplectic coordinate transformation, and hence we cannot use the latent trajectory computed by the transformation $\phi$ in~\eqref{eq:transformation} as a ground truth.
Instead, we compute the ground truth in the latent space by
\begin{equation*}
(y_{true}(s), q_{true}(s)) = 
\varphi_\theta^{-1}(x_{true}(s), p_{true}(s)).   
\end{equation*}
We plot the curves of $(y_{NN}(s), q_{NN}(s))$ and $(y_{true}(s), q_{true}(s))$ parameterized by the time variable $s$ in the right figure of Fig.~\ref{fig:oscillator}. 
We observe that under the learned coordinate transformation $\varphi_\theta$, the latent trajectories are approximately straight lines for both ground truth solution and neural network prediction, and the error is also very small in the latent space. }

\begin{figure}[htbp]
    \centering
    \includegraphics[width=0.8\textwidth]{newfigs/oscillator.pdf}
    \caption{(\textbf{Left}) The solution to~\eqref{eq:HODE}, using the explicit formula~\eqref{eqt:harmonic_ocillator_true_sol} and the prediction given by SympOCNet. It can be seen that the SympOCNet result matches the ground truth well. (\textbf{Right}) We map the curves shown on the left side through the trained SympNet $\varphi_\theta^{-1}$ into the latent space. It can be seen that the latent trajectories are approximately straight lines, and the numerical solution given by SympOCNet fits well to the ground truth.}
    \label{fig:oscillator}
\end{figure}
